# Supplementary material for: Effective and Robust Non-Prehensile Manipulation via Persistent Homology Guided Monte-Carlo Tree Search
Source: arXiv:2210.01283 source file (2024-02-06)
Supplement: Supplementary file 1 [file 10_appendix.tex]

\section{Appendix}
\label{sec:appendix}
